# Supplementary material for: Align and Copy: UZH at SIGMORPHON 2017 Shared Task for Morphological Reinflection
Source: arXiv:1707.01355 ancillary file (2017-07-06)
Supplement: Supplementary file 1 [file supplementary.pdf]

## 1 Supplementary Material

Table 1 summarizes the hyperparameters that we use, which include the dimension $H$ of the LSTM layers, the number of training epochs, and patience. In all the systems, the dimension of the character embedding layer is 100. Throughout, all LSTMs are single-layer. The dimension of the feature embedding layer in HACM is set to 20, and the dimension of the action embedding layer in HAEM is 100. For optimization, we use ADADELTA (Zeiler, 2012) without regularization. All the system are implemented in DyNet (Neubig et al., 2017).

| system | HACM | | | HAEM | | | | Nematus |
|---|---|---|---|---|---|---|---|---|
| setting | low | medium | high | low | medium | high | | |
| | | | | | | rest | naive model 2 | |
| $H$ | 200 | | | | | | 300 | 600 |
| epochs | 50 | 30 | 20 | 60 | 60 | 35 | 20 | 10,000 |
| patience | 10 | 10 | 10 | 30 | 20 | 10 | 10 | 10 |
| dropout | 0.0 | | | 0.5 | | | 0.0 | 0.2 |

Table 1: Hyperparameters and training choices. All HAEM high setting models except model 2 share the same hyperparameters.

**Nematus run** Additionally to the settings documented in Table 1, we use the ADAM optimizer with a learning rate of 0.0001 and batch size 1, and set the length limit on the output sequences per language such that at least 99.5% of all training examples can be represented without truncation. The preprocessing for the character-based Nematus run consists in a) replacing uppercase letters by a sequence of * and the corresponding lowercase characters, b) prefixing all morphological features with the first category (almost always the part-of-speech tag of the lemma). We use tied embeddings (Press and Wolf, 2017), including tying the input and output embeddings of the decoder.

### 1.1 Results on the development set

Tables 2, 3 and 4 show our results on the official development set.

| System | Hard | | Transition | | Hard | | Transition | | Hard & Transition | | | | BS | BS |
|---|---|---|---|---|---|---|---|---|---|---|---|---|---|---|
| Alignment/Run | N | S | N | S | 1 | 2 | 3 | 4 | 5 | 6 | 7 | 7 | | |
| Metric | Acc | Acc | Acc | Acc | Acc | Acc | Acc | Acc | Acc | Acc | Acc | Lev | Acc | Lev |
| albanian | 14.8 | 28.0 | 15.9 | 30.0 | 28.0 | 28.7 | 30.0 | 30.5 | 30.0 | 32.1 | 32.8 | 2.3 | 21.6 | 4.4 |
| arabic | 23.1 | 34.3 | 22.3 | 37.2 | 34.3 | 35.1 | 37.2 | 37.7 | 37.2 | 39.6 | 39.6 | 1.9 | 21.5 | 3.1 |
| armenian | 48.6 | 47.0 | 51.6 | 49.6 | 48.6 | 56.1 | 51.6 | 52.6 | 51.6 | 59.3 | 58.8 | 1.3 | 37.8 | 2.2 |
| basque | 8.0 | 5.0 | 2.0 | 8.0 | 8.0 | 8.0 | 8.0 | 9.0 | 8.0 | 9.0 | 8.0 | 3.8 | 0.0 | 6.5 |
| bengali | 59.0 | 49.0 | 66.0 | 63.0 | 59.0 | 61.0 | 66.0 | 65.0 | 66.0 | 67.0 | 69.0 | 0.6 | 44.0 | 1.5 |
| bulgarian | 44.2 | 46.0 | 46.0 | 51.2 | 46.0 | 47.3 | 51.2 | 53.7 | 51.2 | 55.5 | 54.6 | 0.8 | 33.1 | 1.6 |
| catalan | 59.4 | 59.1 | 62.7 | 63.0 | 59.4 | 60.5 | 63.0 | 62.9 | 63.0 | 64.2 | 64.9 | 0.7 | 55.2 | 1.1 |
| czech | 32.4 | 38.2 | 44.4 | 46.9 | 38.2 | 39.2 | 46.9 | 47.8 | 46.9 | 48.7 | 48.9 | 1.3 | 40.8 | 1.9 |
| danish | 72.1 | 72.6 | 72.9 | 71.7 | 72.6 | 73.0 | 72.9 | 72.9 | 72.9 | 74.5 | 74.4 | 0.4 | 59.8 | 0.7 |
| dutch | 52.2 | 51.7 | 50.8 | 52.8 | 52.2 | 52.4 | 52.8 | 53.3 | 52.8 | 53.2 | 53.1 | 0.7 | 53.7 | 0.7 |
| english | 87.6 | 85.5 | 86.3 | 86.8 | 87.6 | 87.5 | 86.8 | 86.9 | 87.6 | 87.2 | 87.6 | 0.2 | 76.2 | 0.4 |
| estonian | 22.6 | 28.0 | 24.2 | 29.4 | 28.0 | 28.3 | 29.4 | 30.5 | 29.4 | 33.1 | 33.3 | 1.9 | 22.6 | 2.9 |
| faroese | 37.0 | 35.4 | 39.3 | 38.6 | 37.0 | 38.9 | 39.3 | 40.7 | 39.3 | 43.1 | 42.5 | 1.2 | 30.7 | 1.6 |
| finnish | 12.3 | 18.5 | 15.5 | 15.5 | 18.5 | 20.1 | 15.5 | 17.5 | 18.5 | 24.3 | 23.6 | 2.1 | 16.2 | 4.2 |
| french | 66.1 | 60.1 | 64.9 | 65.8 | 66.1 | 67.3 | 65.8 | 66.6 | 66.1 | 67.8 | 68.2 | 0.6 | 63.0 | 0.8 |
| georgian | 81.0 | 69.9 | 81.3 | 78.2 | 81.0 | 79.8 | 81.3 | 81.8 | 81.3 | 81.2 | 83.7 | 0.4 | 71.2 | 0.6 |
| german | 63.9 | 61.3 | 66.8 | 62.4 | 63.9 | 63.8 | 66.8 | 67.7 | 66.8 | 67.1 | 67.3 | 0.8 | 53.7 | 1.1 |
| haida | 45.0 | 2.0 | 45.0 | 3.0 | 45.0 | 45.0 | 45.0 | 45.0 | 45.0 | 47.0 | 47.0 | 2.4 | 34.0 | 6.0 |
| hebrew | 24.2 | 30.5 | 26.2 | 33.9 | 30.5 | 31.5 | 33.9 | 34.4 | 33.9 | 36.0 | 36.2 | 1.1 | 27.9 | 1.3 |
| hindi | 71.9 | 5.4 | 71.1 | 1.0 | 71.9 | 71.9 | 71.1 | 71.1 | 71.9 | 74.5 | 74.6 | 1.0 | 31.0 | 3.8 |
| hungarian | 36.5 | 26.9 | 32.0 | 26.9 | 36.5 | 36.9 | 32.0 | 32.5 | 36.5 | 35.6 | 36.6 | 1.3 | 17.2 | 2.1 |
| icelandic | 39.1 | 33.9 | 40.2 | 36.8 | 39.1 | 39.7 | 40.2 | 40.6 | 40.2 | 41.9 | 42.6 | 1.2 | 34.2 | 1.5 |
| irish | 18.0 | 34.6 | 22.9 | 34.9 | 34.6 | 34.1 | 34.9 | 35.0 | 34.9 | 33.7 | 38.4 | 2.2 | 31.8 | 2.7 |
| italian | 46.8 | 50.8 | 51.6 | 57.6 | 50.8 | 51.8 | 57.6 | 58.4 | 57.6 | 58.2 | 57.8 | 1.0 | 44.9 | 2.0 |
| khaling | 4.0 | 15.0 | 1.4 | 11.3 | 15.0 | 15.4 | 11.3 | 11.0 | 15.0 | 16.3 | 17.2 | 2.6 | 3.9 | 4.3 |
| kurmanji | 85.6 | 84.1 | 86.1 | 85.9 | 85.6 | 86.3 | 86.1 | 86.1 | 86.1 | 87.1 | 86.2 | 0.6 | 82.3 | 0.5 |
| latin | 16.1 | 15.6 | 17.2 | 16.7 | 16.1 | 17.0 | 17.2 | 17.9 | 17.2 | 19.1 | 19.2 | 2.2 | 16.0 | 2.8 |
| latvian | 57.1 | 56.9 | 64.7 | 64.6 | 57.1 | 58.4 | 64.7 | 66.0 | 64.7 | 65.7 | 65.9 | 0.8 | 62.1 | 0.8 |
| lithuanian | 20.0 | 17.3 | 19.9 | 18.7 | 20.0 | 20.6 | 19.9 | 19.5 | 20.0 | 23.1 | 22.9 | 1.8 | 23.5 | 1.9 |
| lower-sorbian | 46.3 | 45.8 | 50.6 | 50.3 | 46.3 | 46.0 | 50.6 | 50.5 | 50.6 | 51.6 | 51.8 | 0.9 | 34.3 | 1.3 |
| macedonian | 57.3 | 47.9 | 57.6 | 57.3 | 57.3 | 58.4 | 57.6 | 58.6 | 57.6 | 61.8 | 62.5 | 0.6 | 50.0 | 1.0 |
| navajo | 5.7 | 16.7 | 8.0 | 18.6 | 16.7 | 16.7 | 18.6 | 18.5 | 18.6 | 18.0 | 19.4 | 3.3 | 18.4 | 3.4 |
| northern-sami | 16.0 | 14.4 | 13.9 | 14.3 | 16.0 | 17.0 | 14.3 | 15.4 | 16.0 | 18.1 | 18.0 | 2.3 | 15.4 | 2.4 |
| norwegian-bokmal | 78.2 | 76.4 | 77.1 | 75.8 | 78.2 | 78.7 | 77.1 | 77.3 | 78.2 | 80.1 | 79.6 | 0.3 | 69.0 | 0.5 |
| norwegian-nynorsk | 50.8 | 47.1 | 53.0 | 50.5 | 50.8 | 51.9 | 53.0 | 53.2 | 53.0 | 54.6 | 54.0 | 0.8 | 50.8 | 0.9 |
| persian | 38.7 | 45.7 | 40.1 | 47.5 | 45.7 | 48.0 | 47.5 | 50.7 | 47.5 | 52.9 | 53.0 | 1.2 | 27.3 | 3.4 |
| polish | 40.4 | 38.3 | 47.1 | 47.1 | 40.4 | 42.0 | 47.1 | 47.4 | 47.1 | 50.2 | 50.3 | 1.4 | 41.9 | 1.6 |
| portuguese | 68.9 | 68.0 | 69.0 | 68.6 | 68.9 | 69.1 | 69.0 | 70.2 | 69.0 | 70.4 | 70.8 | 0.5 | 60.3 | 1.0 |
| quechua | 51.8 | 1.0 | 63.8 | 0.1 | 51.8 | 51.6 | 63.8 | 63.9 | 63.8 | 62.9 | 63.8 | 1.4 | 17.2 | 6.7 |
| romanian | 30.1 | 43.1 | 33.3 | 42.9 | 43.1 | 44.2 | 42.9 | 44.7 | 43.1 | 48.6 | 49.4 | 1.5 | 44.1 | 1.6 |
| russian | 40.3 | 40.7 | 43.2 | 45.1 | 40.7 | 46.1 | 45.1 | 46.4 | 45.1 | 50.1 | 50.6 | 1.2 | 42.8 | 1.3 |
| scottish-gaelic | 44.0 | 62.0 | 54.0 | 78.0 | 62.0 | 64.0 | 78.0 | 78.0 | 78.0 | 70.0 | 78.0 | 0.3 | 48.0 | 0.7 |
| serbo-croatian | 30.4 | 33.2 | 30.2 | 34.5 | 33.2 | 34.3 | 34.5 | 35.2 | 34.5 | 39.0 | 38.3 | 1.7 | 21.3 | 2.7 |
| slovak | 47.4 | 45.6 | 50.0 | 50.5 | 47.4 | 48.6 | 50.5 | 51.9 | 50.5 | 53.2 | 53.5 | 0.8 | 41.9 | 1.0 |
| slovene | 59.0 | 57.2 | 62.3 | 58.7 | 59.0 | 60.1 | 62.3 | 62.1 | 62.3 | 64.4 | 62.9 | 0.6 | 47.4 | 0.9 |
| sorani | 9.2 | 16.9 | 11.6 | 21.6 | 16.9 | 18.2 | 21.6 | 22.4 | 21.6 | 23.3 | 24.0 | 2.2 | 20.5 | 3.4 |
| spanish | 60.2 | 59.0 | 56.9 | 59.7 | 60.2 | 64.3 | 59.7 | 59.1 | 60.2 | 66.6 | 66.3 | 0.7 | 58.6 | 1.2 |
| swedish | 63.7 | 59.0 | 66.6 | 61.9 | 63.7 | 63.8 | 66.6 | 66.7 | 66.6 | 64.3 | 66.6 | 0.5 | 54.3 | 0.9 |
| turkish | 37.4 | 24.1 | 38.4 | 25.5 | 37.4 | 37.2 | 38.4 | 38.1 | 38.4 | 39.7 | 40.8 | 1.7 | 14.3 | 4.3 |
| ukrainian | 41.8 | 41.0 | 42.0 | 41.1 | 41.8 | 42.8 | 42.0 | 42.5 | 42.0 | 45.2 | 45.5 | 1.1 | 40.7 | 1.0 |
| urdu | 64.3 | 60.9 | 68.8 | 67.2 | 64.3 | 66.9 | 68.8 | 69.3 | 68.8 | 72.2 | 71.0 | 0.9 | 30.3 | 4.2 |
| welsh | 48.0 | 42.0 | 54.0 | 46.0 | 48.0 | 48.0 | 54.0 | 55.0 | 54.0 | 57.0 | 57.0 | 0.8 | 15.0 | 1.6 |
| MACRO AVG | 43.8 | 41.3 | 45.8 | 44.3 | 46.5 | 47.6 | 48.9 | 49.5 | 49.2 | 51.1 | 51.6 | 1.3 | 38.0 | 2.1 |

Table 2: Results on low setting for the official development set. N=Naive alignment, S=Smart alignment, BS=Baseline system, Acc=Accuracy, Lev=Levenshtein

| System | Hard | | Transition | | Hard | | Transition | | Hard & Transition | | | | BS | BS |
|---|---|---|---|---|---|---|---|---|---|---|---|---|---|---|
| Alignment/Run | N | S | N | S | 1 | 2 | 3 | 4 | 5 | 6 | 7 | 7 | | |
| Metric | Acc | Acc | Acc | Acc | Acc | Acc | Acc | Acc | Acc | Acc | Acc | Lev | Acc | Lev |
| albanian | 52.7 | 85.4 | 34.6 | 85.0 | 85.4 | 86.4 | 85.0 | 84.7 | 85.4 | 87.4 | 86.7 | 0.3 | 66.1 | 1.2 |
| arabic | 58.9 | 80.1 | 48.9 | 78.4 | 80.1 | 80.3 | 78.4 | 79.1 | 80.1 | 82.2 | 82.1 | 0.5 | 40.0 | 1.8 |
| armenian | 72.0 | 90.9 | 69.8 | 92.3 | 90.9 | 92.0 | 92.3 | 92.5 | 92.3 | 92.9 | 92.6 | 0.1 | 76.6 | 0.4 |
| basque | 73.0 | 75.0 | 41.0 | 74.0 | 75.0 | 76.0 | 74.0 | 75.0 | 75.0 | 79.0 | 78.0 | 0.4 | 2.0 | 5.1 |
| bengali | 98.0 | 96.0 | 99.0 | 96.0 | 98.0 | 98.0 | 99.0 | 99.0 | 99.0 | 98.0 | 99.0 | 0.1 | 75.0 | 0.4 |
| bulgarian | 70.5 | 82.5 | 69.6 | 81.1 | 82.5 | 82.4 | 81.1 | 81.4 | 82.5 | 84.4 | 84.9 | 0.2 | 75.0 | 0.5 |
| catalan | 91.5 | 91.3 | 88.5 | 88.4 | 91.5 | 92.2 | 88.5 | 89.2 | 91.5 | 91.4 | 91.8 | 0.2 | 83.2 | 0.3 |
| czech | 78.0 | 85.9 | 78.0 | 84.3 | 85.9 | 85.9 | 84.3 | 85.3 | 85.9 | 86.7 | 85.9 | 0.3 | 80.7 | 0.4 |
| danish | 83.4 | 82.1 | 82.4 | 81.7 | 83.4 | 83.8 | 82.4 | 82.5 | 83.4 | 83.9 | 84.4 | 0.2 | 78.1 | 0.3 |
| dutch | 81.8 | 81.7 | 79.6 | 80.2 | 81.8 | 84.1 | 80.2 | 82.0 | 81.8 | 84.4 | 85.3 | 0.2 | 71.7 | 0.4 |
| english | 94.4 | 92.1 | 92.8 | 92.0 | 94.4 | 94.1 | 92.8 | 92.8 | 94.4 | 93.6 | 94.4 | 0.1 | 90.2 | 0.2 |
| estonian | 59.6 | 76.4 | 57.4 | 73.6 | 76.4 | 77.8 | 73.6 | 76.7 | 76.4 | 79.6 | 79.3 | 0.4 | 62.4 | 0.8 |
| faroese | 67.3 | 66.9 | 68.2 | 66.4 | 67.3 | 67.4 | 68.2 | 68.3 | 68.2 | 70.1 | 69.9 | 0.6 | 58.7 | 0.9 |
| finnish | 44.7 | 73.1 | 42.0 | 71.7 | 73.1 | 74.1 | 71.7 | 72.4 | 73.1 | 76.7 | 76.5 | 0.4 | 42.5 | 1.4 |
| french | 81.6 | 81.4 | 79.2 | 79.7 | 81.6 | 82.6 | 79.7 | 80.4 | 81.6 | 82.0 | 82.9 | 0.3 | 76.1 | 0.5 |
| georgian | 92.8 | 93.7 | 92.4 | 93.5 | 93.7 | 93.9 | 93.5 | 93.4 | 93.7 | 93.6 | 93.8 | 0.2 | 90.0 | 0.2 |
| german | 80.4 | 80.5 | 79.1 | 79.1 | 80.5 | 80.5 | 79.1 | 79.9 | 80.5 | 80.8 | 81.1 | 0.6 | 71.5 | 0.8 |
| haida | 92.0 | 88.0 | 88.0 | 84.0 | 92.0 | 92.0 | 88.0 | 90.0 | 92.0 | 91.0 | 92.0 | 0.1 | 56.0 | 1.2 |
| hebrew | 75.1 | 81.3 | 51.1 | 73.3 | 81.3 | 82.7 | 73.3 | 73.7 | 81.3 | 82.0 | 82.5 | 0.2 | 40.0 | 0.9 |
| hindi | 89.1 | 96.6 | 89.4 | 97.3 | 96.6 | 96.8 | 97.3 | 97.4 | 97.3 | 97.3 | 97.3 | 0.0 | 86.6 | 0.2 |
| hungarian | 73.1 | 70.7 | 75.3 | 71.7 | 73.1 | 73.4 | 75.3 | 75.0 | 75.3 | 75.4 | 75.3 | 0.5 | 41.7 | 1.6 |
| icelandic | 73.6 | 72.0 | 70.7 | 69.1 | 73.6 | 73.7 | 70.7 | 71.5 | 73.6 | 75.5 | 74.3 | 0.5 | 61.4 | 0.8 |
| irish | 36.6 | 69.8 | 30.6 | 70.5 | 69.8 | 70.1 | 70.5 | 70.7 | 70.5 | 73.2 | 72.6 | 0.8 | 44.7 | 1.5 |
| italian | 84.1 | 93.0 | 77.2 | 92.8 | 93.0 | 93.6 | 92.8 | 92.9 | 93.0 | 93.7 | 93.7 | 0.1 | 73.8 | 0.7 |
| khaling | 68.5 | 78.6 | 9.6 | 69.2 | 78.6 | 79.5 | 69.2 | 69.4 | 78.6 | 80.8 | 80.6 | 0.3 | 18.4 | 1.9 |
| kurmanji | 86.7 | 90.7 | 86.8 | 91.9 | 90.7 | 91.5 | 91.9 | 92.5 | 91.9 | 92.5 | 92.5 | 0.1 | 88.4 | 0.2 |
| latin | 49.6 | 49.0 | 49.0 | 48.9 | 49.6 | 50.5 | 49.0 | 50.2 | 49.6 | 52.9 | 53.2 | 0.8 | 36.8 | 1.1 |
| latvian | 87.6 | 88.4 | 86.6 | 88.2 | 88.4 | 88.3 | 88.2 | 88.2 | 88.4 | 89.0 | 88.6 | 0.2 | 85.1 | 0.3 |
| lithuanian | 58.5 | 59.9 | 58.1 | 58.3 | 59.9 | 60.8 | 58.3 | 60.5 | 59.9 | 62.7 | 62.1 | 0.6 | 53.0 | 0.7 |
| lower-sorbian | 81.2 | 82.5 | 83.1 | 81.8 | 82.5 | 83.4 | 83.1 | 83.1 | 83.1 | 84.0 | 83.1 | 0.4 | 70.5 | 0.6 |
| macedonian | 91.2 | 89.1 | 89.9 | 89.4 | 91.2 | 91.1 | 89.9 | 89.8 | 91.2 | 90.9 | 91.2 | 0.2 | 82.3 | 0.3 |
| navajo | 35.5 | 48.8 | 10.6 | 37.5 | 48.8 | 50.0 | 37.5 | 37.6 | 48.8 | 49.7 | 50.4 | 1.4 | 31.3 | 2.5 |
| northern-sami | 65.5 | 65.1 | 53.9 | 61.8 | 65.5 | 68.4 | 61.8 | 63.6 | 65.5 | 71.3 | 71.7 | 0.5 | 35.7 | 1.5 |
| norwegian-bokmal | 83.2 | 83.1 | 83.2 | 83.5 | 83.2 | 83.3 | 83.5 | 83.2 | 83.5 | 83.7 | 83.8 | 0.2 | 79.8 | 0.3 |
| norwegian-nynorsk | 67.8 | 66.5 | 67.3 | 67.5 | 67.8 | 68.3 | 67.5 | 68.1 | 67.8 | 69.7 | 69.3 | 0.5 | 63.3 | 0.6 |
| persian | 71.5 | 86.9 | 63.0 | 83.2 | 86.9 | 87.0 | 83.2 | 83.7 | 86.9 | 88.1 | 88.1 | 0.2 | 65.4 | 1.1 |
| polish | 77.3 | 80.8 | 74.7 | 78.8 | 80.8 | 80.8 | 78.8 | 80.0 | 80.8 | 82.4 | 82.5 | 0.4 | 75.2 | 0.5 |
| portuguese | 94.4 | 94.3 | 93.1 | 93.8 | 94.4 | 94.2 | 93.8 | 93.8 | 94.4 | 94.5 | 94.4 | 0.1 | 92.9 | 0.1 |
| quechua | 96.9 | 95.7 | 97.3 | 95.2 | 96.9 | 98.3 | 97.3 | 98.7 | 97.3 | 99.2 | 99.0 | 0.0 | 68.1 | 1.7 |
| romanian | 62.9 | 78.5 | 60.1 | 76.2 | 78.5 | 79.2 | 76.2 | 77.4 | 78.5 | 79.6 | 79.5 | 0.7 | 70.2 | 0.9 |
| russian | 78.4 | 83.7 | 77.0 | 81.8 | 83.7 | 84.2 | 81.8 | 82.2 | 83.7 | 84.1 | 84.9 | 0.4 | 75.0 | 0.7 |
| scottish-gaelic | 94.0 | 92.0 | 92.0 | 92.0 | 94.0 | 94.0 | 92.0 | 94.0 | 94.0 | 92.0 | 94.0 | 0.1 | 52.0 | 0.8 |
| serbo-croatian | 67.9 | 83.2 | 67.1 | 83.7 | 83.2 | 84.1 | 83.7 | 83.6 | 83.7 | 85.0 | 85.0 | 0.3 | 65.8 | 0.9 |
| slovak | 79.6 | 79.2 | 78.6 | 78.6 | 79.6 | 80.1 | 78.6 | 79.4 | 79.6 | 81.5 | 81.4 | 0.3 | 70.7 | 0.5 |
| slovene | 86.2 | 87.2 | 86.8 | 87.1 | 87.2 | 87.3 | 87.1 | 87.7 | 87.2 | 87.6 | 88.1 | 0.2 | 81.9 | 0.3 |
| sorani | 58.3 | 71.8 | 26.6 | 65.9 | 71.8 | 73.1 | 65.9 | 67.1 | 71.8 | 75.8 | 75.4 | 0.4 | 52.8 | 1.1 |
| spanish | 80.9 | 90.7 | 80.8 | 89.0 | 90.7 | 90.9 | 89.0 | 89.5 | 90.7 | 90.8 | 91.1 | 0.2 | 85.4 | 0.3 |
| swedish | 77.5 | 77.8 | 80.3 | 79.9 | 77.8 | 78.9 | 80.3 | 80.2 | 80.3 | 79.9 | 80.3 | 0.3 | 73.7 | 0.5 |
| turkish | 89.4 | 83.6 | 89.1 | 84.4 | 89.4 | 89.4 | 89.1 | 90.0 | 89.4 | 91.2 | 90.9 | 0.2 | 33.1 | 2.9 |
| ukrainian | 77.7 | 79.9 | 79.0 | 79.8 | 79.9 | 79.2 | 79.8 | 79.9 | 79.9 | 80.7 | 80.3 | 0.4 | 71.5 | 0.5 |
| urdu | 87.7 | 96.6 | 87.8 | 97.4 | 96.6 | 97.0 | 97.4 | 97.4 | 97.4 | 97.7 | 97.5 | 0.0 | 86.1 | 0.3 |
| welsh | 82.0 | 82.0 | 78.0 | 77.0 | 82.0 | 86.0 | 78.0 | 80.0 | 82.0 | 87.0 | 87.0 | 0.2 | 54.0 | 1.0 |
| MACRO AVG | 75.8 | 81.4 | 70.7 | 80.0 | 81.9 | 82.6 | 80.5 | 81.1 | 82.2 | 83.4 | 83.5 | 0.3 | 64.7 | 0.9 |

Table 3: Results on medium setting for the official development set. N=Naive alignment, S=Smart alignment, BS=Baseline system, Acc=Accuracy, Lev=Levenshtein

| System | Hard | | Transition | | Hard | | Transition | | Hard & Transition & Nematus | | | | BS | BS |
|---|---|---|---|---|---|---|---|---|---|---|---|---|---|---|
| Alignment/Run | N | S | N | S | 1 | 2 | 3 | 4 | 5 | 6 | 7 | 7 | | |
| Metric | Acc | Acc | Acc | Acc | Acc | Acc | Acc | Acc | Acc | Acc | Acc | Lev | Acc | Lev |
| albanian | 96.4 | 96.0 | 39.8 | 93.3 | 96.4 | 97.2 | 93.3 | 94.4 | 99.1 | 97.6 | 99.1 | 0.0 | 78.1 | 0.6 |
| arabic | 93.8 | 93.5 | 51.0 | 88.0 | 93.8 | 95.0 | 88.0 | 87.4 | 94.9 | 95.0 | 95.4 | 0.2 | 47.7 | 1.5 |
| armenian | 94.8 | 96.5 | 72.4 | 96.8 | 96.5 | 97.4 | 96.8 | 96.7 | 97.6 | 97.7 | 97.6 | 0.1 | 89.1 | 0.2 |
| basque | 100.0 | 99.0 | 47.0 | 97.0 | 100.0 | 99.0 | 97.0 | 95.0 | 100.0 | 99.0 | 100.0 | 0.0 | 6.0 | 3.3 |
| bengali | 99.0 | 99.0 | 99.0 | 99.0 | 99.0 | 99.0 | 99.0 | 99.0 | 99.0 | 99.0 | 99.0 | 0.0 | 84.0 | 0.3 |
| bulgarian | 96.6 | 97.0 | 78.1 | 95.9 | 97.0 | 97.5 | 95.9 | 95.6 | 97.4 | 97.8 | 97.7 | 0.0 | 90.0 | 0.2 |
| catalan | 97.8 | 97.5 | 95.6 | 96.5 | 97.8 | 97.9 | 96.5 | 97.1 | 98.1 | 97.9 | 98.1 | 0.1 | 94.2 | 0.1 |
| czech | 90.5 | 94.0 | 84.1 | 91.8 | 94.0 | 94.4 | 91.8 | 92.7 | 94.0 | 94.4 | 94.4 | 0.1 | 90.4 | 0.2 |
| danish | 95.7 | 94.3 | 84.8 | 83.7 | 95.7 | 95.6 | 84.8 | 84.8 | 95.7 | 95.2 | 95.7 | 0.1 | 89.1 | 0.2 |
| dutch | 95.4 | 96.6 | 88.3 | 93.0 | 96.6 | 97.0 | 93.0 | 93.2 | 97.1 | 97.1 | 97.3 | 0.0 | 86.8 | 0.2 |
| english | 96.1 | 96.4 | 93.5 | 94.3 | 96.4 | 96.3 | 94.3 | 94.3 | 96.4 | 96.3 | 96.4 | 0.1 | 95.0 | 0.1 |
| estonian | 97.8 | 97.3 | 65.6 | 92.7 | 97.8 | 98.1 | 92.7 | 93.4 | 98.8 | 98.3 | 98.8 | 0.0 | 76.2 | 0.5 |
| faroese | 87.3 | 85.9 | 71.1 | 72.2 | 87.3 | 88.0 | 72.2 | 73.8 | 87.3 | 87.5 | 88.2 | 0.3 | 74.7 | 0.6 |
| finnish | 83.0 | 93.4 | 52.6 | 88.2 | 93.4 | 94.0 | 88.2 | 89.1 | 93.7 | 94.2 | 94.3 | 0.1 | 78.5 | 0.4 |
| french | 90.0 | 90.9 | 81.5 | 83.0 | 90.9 | 91.9 | 83.0 | 84.0 | 90.9 | 91.1 | 91.9 | 0.1 | 83.6 | 0.3 |
| georgian | 98.3 | 98.7 | 95.8 | 98.0 | 98.7 | 99.1 | 98.0 | 98.5 | 98.7 | 99.2 | 99.0 | 0.0 | 94.0 | 0.1 |
| german | 89.7 | 89.8 | 81.5 | 83.6 | 89.8 | 90.6 | 83.6 | 83.8 | 89.9 | 90.1 | 92.1 | 0.2 | 81.2 | 0.6 |
| haida | 99.0 | 98.0 | 98.0 | 98.0 | 99.0 | 99.0 | 98.0 | 99.0 | 99.0 | 99.0 | 99.0 | 0.0 | 69.0 | 0.6 |
| hebrew | 98.6 | 98.5 | 59.1 | 96.8 | 98.6 | 98.8 | 96.8 | 94.5 | 98.6 | 98.8 | 99.0 | 0.0 | 55.8 | 0.6 |
| hindi | 99.3 | 100.0 | 91.2 | 100.0 | 100.0 | 100.0 | 100.0 | 99.9 | 100.0 | 100.0 | 100.0 | 0.0 | 94.0 | 0.1 |
| hungarian | 87.1 | 86.0 | 78.1 | 81.5 | 87.1 | 87.4 | 81.5 | 82.6 | 87.4 | 88.0 | 87.8 | 0.3 | 71.1 | 0.6 |
| icelandic | 91.8 | 90.3 | 83.0 | 83.5 | 91.8 | 92.1 | 83.5 | 85.5 | 91.8 | 91.8 | 92.3 | 0.2 | 76.1 | 0.5 |
| irish | 65.1 | 91.7 | 31.6 | 86.8 | 91.7 | 92.1 | 86.8 | 86.5 | 91.7 | 92.3 | 92.4 | 0.2 | 54.3 | 1.1 |
| italian | 97.1 | 97.0 | 79.8 | 96.3 | 97.1 | 97.3 | 96.3 | 96.3 | 97.7 | 97.4 | 97.7 | 0.1 | 79.9 | 0.6 |
| khaling | 98.5 | 99.3 | 15.9 | 90.9 | 99.3 | 99.6 | 90.9 | 89.5 | 99.3 | 99.6 | 99.8 | 0.0 | 53.8 | 0.8 |
| kurmanji | 93.0 | 93.9 | 87.2 | 94.3 | 93.9 | 93.8 | 94.3 | 94.4 | 94.3 | 94.1 | 94.3 | 0.1 | 92.2 | 0.1 |
| latin | 81.8 | 80.7 | 56.2 | 58.4 | 81.8 | 81.9 | 58.4 | 60.1 | 81.8 | 80.3 | 81.9 | 0.3 | 45.6 | 0.9 |
| latvian | 93.7 | 97.0 | 90.3 | 95.2 | 97.0 | 97.2 | 95.2 | 95.4 | 97.0 | 97.0 | 97.3 | 0.0 | 91.0 | 0.3 |
| lithuanian | 91.6 | 92.1 | 76.1 | 84.2 | 92.1 | 93.3 | 84.2 | 85.3 | 92.6 | 92.8 | 93.6 | 0.1 | 64.7 | 0.5 |
| lower-sorbian | 97.4 | 97.0 | 95.3 | 95.8 | 97.4 | 97.5 | 95.8 | 96.4 | 97.4 | 97.4 | 97.5 | 0.1 | 86.0 | 0.3 |
| macedonian | 95.2 | 95.9 | 93.0 | 94.5 | 95.9 | 96.1 | 94.5 | 94.3 | 95.9 | 96.0 | 96.3 | 0.1 | 91.9 | 0.2 |
| navajo | 84.2 | 88.1 | 9.8 | 60.4 | 88.1 | 90.6 | 60.4 | 60.4 | 89.1 | 91.1 | 91.6 | 0.2 | 38.3 | 2.1 |
| northern-sami | 96.3 | 95.8 | 69.0 | 83.4 | 96.3 | 97.0 | 83.4 | 84.3 | 96.9 | 97.1 | 97.2 | 0.1 | 61.1 | 0.8 |
| norwegian-bokmal | 92.4 | 92.2 | 84.5 | 85.1 | 92.4 | 93.1 | 85.1 | 85.3 | 92.4 | 92.7 | 93.0 | 0.1 | 90.6 | 0.2 |
| norwegian-nynorsk | 94.2 | 92.3 | 71.0 | 70.5 | 94.2 | 94.3 | 71.0 | 72.5 | 94.2 | 93.6 | 94.4 | 0.1 | 78.3 | 0.4 |
| persian | 99.3 | 98.9 | 68.2 | 92.5 | 99.3 | 99.5 | 92.5 | 93.1 | 99.4 | 99.5 | 99.6 | 0.0 | 77.6 | 0.6 |
| polish | 89.3 | 92.4 | 84.4 | 90.1 | 92.4 | 93.0 | 90.1 | 90.7 | 92.4 | 93.0 | 93.4 | 0.1 | 89.4 | 0.2 |
| portuguese | 99.0 | 99.0 | 97.8 | 98.5 | 99.0 | 99.0 | 98.5 | 98.3 | 99.0 | 99.0 | 99.2 | 0.0 | 97.4 | 0.0 |
| quechua | 98.9 | 99.4 | 98.1 | 99.7 | 99.4 | 99.9 | 99.7 | 99.9 | 99.7 | 99.9 | 99.9 | 0.0 | 94.7 | 0.1 |
| romanian | 81.8 | 88.4 | 62.7 | 82.4 | 88.4 | 88.3 | 82.4 | 82.5 | 88.4 | 88.7 | 88.4 | 0.4 | 80.4 | 0.7 |
| russian | 87.2 | 92.3 | 82.1 | 90.2 | 92.3 | 93.1 | 90.2 | 90.6 | 92.3 | 92.5 | 92.6 | 0.3 | 82.0 | 0.6 |
| scottish-gaelic | n/a | n/a | n/a | n/a | n/a | n/a | n/a | n/a | n/a | n/a | n/a | n/a | n/a | n/a |
| serbo-croatian | 82.3 | 92.5 | 72.3 | 90.9 | 92.5 | 92.3 | 90.9 | 91.0 | 92.5 | 92.3 | 92.7 | 0.2 | 84.0 | 0.4 |
| slovak | 96.7 | 96.4 | 89.9 | 88.3 | 96.7 | 96.6 | 89.9 | 90.6 | 96.7 | 96.8 | 96.7 | 0.1 | 85.2 | 0.3 |
| slovene | 96.9 | 97.2 | 93.9 | 95.9 | 97.2 | 97.6 | 95.9 | 96.5 | 97.9 | 98.0 | 97.9 | 0.0 | 89.8 | 0.2 |
| sorani | 89.7 | 90.5 | 30.7 | 80.8 | 90.5 | 91.8 | 80.8 | 81.3 | 90.5 | 92.1 | 91.5 | 0.1 | 64.3 | 0.7 |
| spanish | 96.1 | 96.7 | 83.6 | 94.3 | 96.7 | 97.1 | 94.3 | 94.3 | 96.9 | 96.6 | 97.0 | 0.1 | 90.6 | 0.2 |
| swedish | 90.8 | 91.2 | 83.2 | 83.1 | 91.2 | 91.5 | 83.2 | 83.8 | 91.2 | 91.4 | 92.3 | 0.2 | 85.4 | 0.3 |
| turkish | 98.2 | 96.1 | 97.8 | 94.6 | 98.2 | 97.7 | 97.8 | 97.4 | 98.2 | 97.4 | 98.2 | 0.0 | 72.9 | 0.8 |
| ukrainian | 94.2 | 93.9 | 88.1 | 90.8 | 94.2 | 94.6 | 90.8 | 91.5 | 94.2 | 94.9 | 94.7 | 0.1 | 86.3 | 0.3 |
| urdu | 99.5 | 99.7 | 89.3 | 99.5 | 99.7 | 99.5 | 99.5 | 99.6 | 99.7 | 99.6 | 99.7 | 0.0 | 95.8 | 0.1 |
| welsh | 100.0 | 99.0 | 98.0 | 97.0 | 100.0 | 100.0 | 98.0 | 98.0 | 100.0 | 100.0 | 100.0 | 0.0 | 67.0 | 0.5 |
| MACRO AVG | 93.3 | 94.6 | 75.9 | 89.6 | 95.0 | 95.3 | 89.8 | 90.1 | 95.2 | 95.3 | 95.6 | 0.1 | 77.9 | 0.5 |

Table 4: Results on high setting (including a run of the Nematus systems) for the official development set. N=Naive alignment, S=Smart alignment, BS=Baseline system, Acc=Accuracy, Lev=Levenshtein

## References


Graham Neubig, Chris Dyer, Yoav Goldberg, Austin Matthews, Waleed Ammar, Antonios Anastasopoulos, Miguel Ballesteros, David Chiang, Daniel Clothiaux, Trevor Cohn, Kevin Duh, Manaal Faruqui, Cynthia Gan, Dan Garrette, Yangfeng Ji, Lingpeng Kong, Adhiguna Kuncoro, Gaurav Kumar, Chaitanya Malaviya, Paul Michel, Yusuke Oda, Matthew Richardson, Naomi Saphra, Swabha Swayamdipta, and Pengcheng Yin. 2017. DyNet: The Dynamic Neural Network Toolkit. *arXiv preprint arXiv:1701.03980* .

Ofir Press and Lior Wolf. 2017. Using the output embedding to improve language models. In *ACL*.

Matthew D Zeiler. 2012. ADADELTA: an adaptive learning rate method. arXiv:1212.5701.
